# Supplementary material for: Self-Supervised Graph Learning with Hyperbolic Embedding for Temporal Health Event Prediction
Source: arXiv:2106.04751 source file (2021-12-05)
Supplement: Supplementary file 1 [file appendix.tex]

% \section{Algorithms}
% \label{sec:appendix_algo}

% Two procedures, \texttt{HyperbolicEmbedding} and \texttt{Encoder}, used in Algorithm~\ref{algo:model_algo} are described as follows:

% \begin{procedure}
%     \DontPrintSemicolon
%     \SetAlgoLined
%     % \SetAlgorithmName{Procedure}{Procedure}{Procedure}
%     \SetKwInOut{Input}{Input}
%     \SetKwInOut{Output}{Output}

%     \Input{The hierarchical structure $\mathcal{H}$ of medical codes}
%     \Output{Embeddings $\mathbf{E}$ for leaf nodes of $\mathcal{H}$}
%     Randomly initialize shared and local vectors \\
%     \For{$c_i \in \mathcal{H}$}{
%         $\mathbf{e}'_i \leftarrow$ combine shared and local vector $\mathbf{s}_i, \mathbf{t}_i$ \\
%         $\mathbf{s}'_i, \mathbf{t}'_i \leftarrow$ Downward and upward flow \\
%         $\mathbf{e}_i \leftarrow$ combine $\mathbf{s}'_i, \mathbf{t}'_i$ \\
%     }
%     \Repeat{convergence}{
%         Calculate distance by Equation~(\ref{eq:hyperbolic_dist}) \\
%         Optimizing embedding vectors using $\mathcal{L}_{\text{rec}}$ \\
%     }
%     \Return $\{\mathbf{e}_i \mid \text{$c_i$ is a leaf node in $\mathcal{H}$}\}$
%     \caption{HyperbolicEmbedding($\mathcal{H}$)}
%     \label{algo:hyperbolic_algo}
% \end{procedure}

% \begin{procedure}
%     \DontPrintSemicolon
%     \SetAlgoLined
%     % \SetAlgorithmName{Procedure}{Procedure}{Procedure}
%     \SetKwInOut{Input}{Input}
%     \SetKwInOut{Output}{Output}

%     \Input{A patient $u$, an EHR dataset $\mathcal{D}$, the GNN output of medical code embeddings $\mathbf{X}$}
%     \Output{The patient embedding vector $\mathbf{p}$ of $u$}
%     $V_1, V_2, \dots, V_{T} \leftarrow$ Get admission records of $u$ from $\mathcal{D}$ \\
%     \For{$\tau \leftarrow 1$ to $T$}{
%         $\mathbf{v}_\tau \leftarrow$ Calculate the admission embedding using code-level attention with $\mathbf{X}$ \\
%     }
%     $\mathbf{p} \leftarrow$ Calculate the patient embedding using admission-level attention \\
%     \Return $\mathbf{p}$
%     \caption{Encoder($u, \mathcal{D}, \mathbf{X}$)}
%     \label{algo:encoder_algo}
% \end{procedure}

% \section{Parameter Settings for Baselines}
% The detailed parameter setting for baselines compared in Section~\ref{sec:experiments} are given as follows:
% \begin{itemize}[leftmargin=*]
%     \item \dnn: The hidden units for two hidden layers are 128 and 64, respectively.
%     \item \doctorai: The hidden size for the RNN layer is 128.
%     \item \retain: The embedding size for admissions is 256. The hidden layer size for two RNN layers is 128.
%     \item \deepr: The embedding size for medical codes is 100. The kernel size and filter num for an 1-D CNN layer are 3 and 128, respectively.
%     \item \gram: The embedding size for medical codes is 100. The attention size is 100. The hidden size for the RNN layer is 128.
%     \item \dipole: The embedding size for admissions is 256. The concatenation-based attention size is 128. The hidden size for the RNN layer is 128.
%     \item \timeline: The embedding size for medical codes is 100. The attention size is 100. The hidden size for the RNN layer is 128.
%     \item \gbert: The parameter settings are the same as ~\cite{shang2019pretrain}. (1) GAT part: The input embedding size is 75, the number of attention heads is 4; (2) BERT part: the hidden size is 300, the dimension of position-wise feed-forward networks as 300, 2 hidden layers with 4 attention heads for each layer.
% \end{itemize}
% \label{sec:appendix_param}
